# Supplementary material for: A Framework for the Analysis of Computational Imaging Systems with Practical Applications
Source: arXiv:1308.1981 source file (2014-03-13)
Supplement: Supplementary file 1 [file AppendixA.tex]

We show that the MMSE can be written as the sum of two terms: an intra-mixture error term and an inter-mixture error term, see Eqn. \eqref{eqn:GMM_MSE}. The original expression of MMSE is given by Eqn. \eqref{eq:GMMMSEDef}. Let us first concentrate on the inner integral in Eqn. \eqref{eq:GMMMSEDef}:

\begin{equation}
\int_x ||x-\hat{x}(y)||^2 P(x|y)\textrm{d}x.  
\label{eq:innerInt}
\end{equation}
Using the expression for $P(x|y)$ in Eqn. \eqref{eq:GMMposterior}, the above integral can be written as

\begin{equation}
\sum_{k=1}^K \widetilde{\alpha_k}(y) \int_x ||x-\hat{x}(y)||^2 P_k(x|y)\textrm{d}x. \nonumber
\end{equation}
We then add and subtract $\widetilde{m_k}(y)$ to obtain

\begin{equation}
\begin{split}
\sum_{k=1}^K \widetilde{\alpha_k}(y) \int_x ||x-\widetilde{m_k}(y) + \widetilde{m_k}(y)-\hat{x}(y)||^2 P_k(x|y)\textrm{d}x. \nonumber
\end{split}
\end{equation}
Using the expansion $||a+b||^2=||a||^2+||b||^2+2a^Tb$ with $a=x-\widetilde{m_k}(y)$ and $b=\widetilde{m_k}(y)-\hat{x}(y)$  and keeping in mind that the term $b$ is independent of $x$, we get

\begin{equation}
\begin{split}
\sum_{k=1}^K \widetilde{\alpha_k}(y)\int_x ||x-\widetilde{m_k}(y)||^2 P_k(x|y)\textrm{d}x \nonumber\\ 
+\sum_{k=1}^K \widetilde{\alpha_k}(y) ||\widetilde{m_k}(y)-\hat{x}(y)||^2 \nonumber\\
+\sum_{k=1}^K \widetilde{\alpha_k}(y) (\widetilde{m_k}(y)-\hat{x}(y))^T \int_x (x-\widetilde{m_k}(y)) P_k(x|y)\textrm{d}x. \nonumber
\end{split}
\end{equation}
Since, $P_k(x|y)$ is a Gaussian distribution with mean $\widetilde{m_k}(y)$ and covariance $\widetilde{\Sigma_k}$, see Eqn. \eqref{eq:GMMGaussians}, we can rewrite the above expression as

\begin{equation}
\sum_{k=1}^K \widetilde{\alpha_k}(y)Tr(\widetilde{\Sigma_k})+\sum_{k=1}^K \widetilde{\alpha_k}(y) ||\widetilde{m_k}(y)-\hat{x}(y)||^2. \nonumber
\end{equation}
Thus, till now, we have shown that the inner integral of the MMSE, Eqn. \eqref{eq:innerInt}, is given by the above expression. Now we consider the outer integral in Eqn. \eqref{eq:GMMMSEDef}.

Taking the outer integral into account, the MMSE can be written as

\begin{equation}
\begin{split}
\sum_{k=1}^K Tr(\widetilde{\Sigma_k}) \int_y \widetilde{\alpha_k}(y) P(y) \textrm{d}y \nonumber\\
+\sum_{k=1}^K \int_y ||\widetilde{m_k}(y)-\hat{x}(y)||^2 \widetilde{\alpha_k}(y) P(y) \textrm{d}y. \nonumber
\end{split}
\end{equation}
Using the definitions of $\widetilde{\alpha_k}(y)$ , Eqn. \eqref{eq:posteriorWt}, and $P(y)$, Eqn. \eqref{eq:marginalObs}, we can rewrite the above expression as

\begin{equation}
\sum_{k=1}^K \alpha_k Tr(\widetilde{\Sigma_k}) + \sum_{k=1}^K \alpha_k \int_y ||\widetilde{m_k}(y)-\hat{x}(y)||^2 P_k(y) \textrm{d}y, \nonumber
\end{equation}
which expresses the MMSE as the sum of the intra-mixture and inter-mixture terms, as in Eqn. \eqref{eqn:GMM_MSE}. 
